# Supplementary material for: Opening up the Quantum Three-Box Problem with Undetectable Measurements
Source: arXiv:1205.2594 source file (2012-05-11)
Supplement: Supplementary file 1 [file 3box-supplement.pdf]

# Supporting Information for: Opening up the Quantum Three-Box Problem with Undetectable Measurements

Richard E. George,[1,*] Lucio Robledo,[2,†] Owen Maroney,[3] Machiel Blok,[2] Hannes Bernien,[2] Matthew L. Markham,[4] Daniel J. Twitchen,[4] John J. L. Morton,[1] G. Andrew D. Briggs,[1] and Ronald Hanson[2]

[1] *University of Oxford, Department of Materials, 12/13 Parks Road, Oxford, OX1 3PH, United Kingdom*

[2] *Kavli Institute of Nanoscience Delft, Delft University of Technology, Post Office Box 5046, 2600 GA Delft, The Netherlands*

[3] *Faculty of Oxford, Department of Philosophy, 10 Merton Street, Oxford, OX1 4JJ, United Kingdom*

[4] *Element Six, Ltd., Kings Ride Park, Ascot, Berkshire SL5 8BP, United Kingdom*

(Dated: May 10, 2012)

In this document, we detail the projections performed by Bob's measurements, and provide a detailed account of the states prepared during the experiment. We detail how Alice is able to transform her initial state $|3\rangle$ into the state $|I\rangle$, and subsequently transform $|F\rangle$ back onto state $|3\rangle$. We describe our notation for probabilities that allow us to describe the 'three-box' game both from a classical and quantum perspective. We derive the Leggett-Garg function for this system as calculated by an observer who assumes the system obeys the axioms of macrorealism, namely state definiteness and non invasive measurability. We describe the sample fabrication and measurement setup, and discuss the practicalities of the experimental measurements involving reading out the nuclear spin, and discuss the significance of finite measurement precision and of measurement errors.

**Projections performed by Bob's measurements**

In the main text of the letter, we state that Bob finding a measurement result $M_j$-true prepares the state $|j\rangle$ by performing projector $\hat{P}_j$ on state $|I\rangle$, while him finding the result $M_j$-false prepares an orthogonal state $|\psi_j'\rangle$ by performing projector $\hat{P}_j^{\perp}$. Here, we give explicit vector representations of these states, and matrix representations of the projectors $\hat{P}_j$ and $\hat{P}_j^{\perp}$, to aid understanding. We can write a column vector to represent the general state $|\psi\rangle$ of the 'three box' problem as:

$$|\psi\rangle = a\,|1\rangle + b\,|2\rangle + c\,|3\rangle = \begin{pmatrix} a \\ b \\ c \end{pmatrix} \tag{1}$$

The initial and final states used by Alice are then written:

$$|I\rangle = \frac{1}{\sqrt{3}} \begin{pmatrix} 1 \\ 1 \\ 1 \end{pmatrix} \qquad\qquad \langle F| = \frac{1}{\sqrt{3}} \begin{pmatrix} 1 & 1 & -1 \end{pmatrix} \tag{2}$$

We write the identity matrix as:

$$\mathbb{1} = \sum_j |j\rangle\langle j| = \begin{pmatrix} 1 & 0 & 0 \\ 0 & 1 & 0 \\ 0 & 0 & 1 \end{pmatrix} \tag{3}$$

and write the projectors $\hat{P}_j$ and $\hat{P}_j^{\perp}$ explicitly as:

$$\hat{P}_1 = |1\rangle\langle 1| = \begin{pmatrix} 1 & 0 & 0 \\ 0 & 0 & 0 \\ 0 & 0 & 0 \end{pmatrix} \qquad \hat{P}_1^{\perp} = \mathbb{1} - \hat{P}_1 = |2\rangle\langle 2| + |3\rangle\langle 3| = \begin{pmatrix} 0 & 0 & 0 \\ 0 & 1 & 0 \\ 0 & 0 & 1 \end{pmatrix} \tag{4}$$

$$\hat{P}_2 = |2\rangle\langle 2| = \begin{pmatrix} 0 & 0 & 0 \\ 0 & 1 & 0 \\ 0 & 0 & 0 \end{pmatrix} \qquad \hat{P}_2^{\perp} = \mathbb{1} - \hat{P}_2 = |1\rangle\langle 1| + |3\rangle\langle 3| = \begin{pmatrix} 1 & 0 & 0 \\ 0 & 0 & 0 \\ 0 & 0 & 1 \end{pmatrix} \tag{5}$$

Using this representation it is straightforward to verify the claims in the main text, that:

$$P_{M_1}(A \cap B) = |\langle F|\hat{P}_1|I\rangle|^2 = P_{M_2}(A \cap B) = |\langle F|\hat{P}_2|I\rangle|^2 = 1/9 \tag{6}$$

$$P_{M_1}(A \cap \neg B) = |\langle F|\hat{P}_1^{\perp}|I\rangle|^2 = P_{M_2}(A \cap \neg B) = |\langle F|\hat{P}_2^{\perp}|I\rangle|^2 = 0 \tag{7}$$

These expressions describe Alice's ability to win $\gg 50\%$ of rounds in the quantum version of the game.

## ALICE'S UNITARY OPERATIONS

### Preparing the initial state

Alice would like to measure $|I\rangle$ and $|F\rangle$, but only has access to $M_3$. She performs effective $M_I$ and $M_F$ measurements by performing unitaries that map $|I\rangle \to |3\rangle$ and $|F\rangle \to |3\rangle$, followed by $M_3$ measurement. We define the unitary operation applied by Alice to transform between the states $|3\rangle$ and $|I\rangle$ in terms of it's ability to split a population initially prepared in level $|3\rangle$ into an equal superposition of the states $|1\rangle$, $|2\rangle$ and $|3\rangle$. We construct $\hat{U}_I$ by concatenating two unitaries that can be implemented as RF pulses. The first step in performing $\hat{U}_I$ represents a rotation through angle $\theta$ in the $\{|3\rangle, |2\rangle\}$ plane, and the second step represents a rotation through angle $90^{\circ} = \pi/2$ in the $\{|3\rangle, |1\rangle\}$ plane.

The first rotation ($\theta$ in the $\{|3\rangle, |1\rangle\}$ plane) must transfer 1/3 of the population from state $|3\rangle$ to state $|1\rangle$, leaving 2/3 of the population in state $|3\rangle$. The subsequent rotation must split the population in level $|3\rangle$ equally between $|3\rangle$ and $|2\rangle$, producing an equal population of 1/3 in each of the three $|j\rangle$ states.

Considering the coherent rotation in the $\{|3\rangle, |1\rangle\}$ plane, a rotation through $\theta$ transfers a fraction $\sin^2(\theta/2)$ into state $|1\rangle$ whilst leaving a fraction $\cos^2(\theta/2)$ in state $|3\rangle$, so to place 1/3 of the population in state $|1\rangle$, we have:

$$\sin^2(\theta/2) = 1/3 \qquad \cos^2(\theta/2) = 2/3 \tag{8}$$

Implying that:

$$\sin(\theta/2) = \sqrt{1/3} \qquad \cos(\theta/2) = \sqrt{2/3} \tag{9}$$

$$\tan(\theta/2) = \sqrt{1/2} \qquad \theta = 2\tan^{-1}(\sqrt{1/2}) \tag{10}$$

with the result that:

$$\theta = 70.6^\circ \; (= 1.23 \text{ radians}) \tag{11}$$

Alice prepares state $|3\rangle$ and performs $\hat{U}_I$ as two rotations: $\theta = 70.6^\circ$ in the $\{|3\rangle, |1\rangle\}$ plane and $\pi/2 = 90^\circ$ in the $\{|3\rangle, |2\rangle\}$ plane.

**Alice's measurement of $|F\rangle$**

The states $|I\rangle$ and $|F\rangle$ are defined in Vaidman's paper as:

$$|I\rangle = \frac{|1\rangle + |2\rangle + |3\rangle}{\sqrt{3}} \qquad |F\rangle = \frac{|1\rangle + |2\rangle - |3\rangle}{\sqrt{3}} \tag{12}$$

Since quantum states are defined only up to an overall multiplicative scalar (states such as $|F\rangle$ are rays in the Hilbert space), we can choose to write:

$$|F\rangle = \frac{-|1\rangle - |2\rangle + |3\rangle}{\sqrt{3}} \tag{13}$$

A rotation through $2\pi$ radians introduces a sign change, so that two combined rotations through $2\pi$, first on the $\{|3\rangle, |1\rangle\}$ and then the $\{|3\rangle, |2\rangle\}$ levels. We have:

$$\begin{pmatrix} |1'\rangle \\ |3'\rangle \\ |2'\rangle \end{pmatrix} = \underbrace{\begin{pmatrix} 1 & 0 & 0 \\ 0 & -1 & 0 \\ 0 & 0 & -1 \end{pmatrix} \begin{pmatrix} -1 & 0 & 0 \\ 0 & -1 & 0 \\ 0 & 0 & 1 \end{pmatrix}}_{\hat{U}_{IF}} \begin{pmatrix} |1\rangle \\ |3\rangle \\ |2\rangle \end{pmatrix} \tag{14}$$

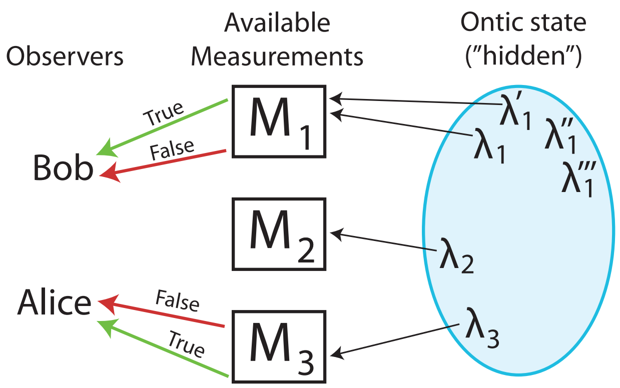


FIG. 1. **A classical model of the three-box problem.** In a simple classical model, the system is assumed to exist in a definite state $\lambda_j$. The specific state $\lambda_j$ then determines how the system will respond to each measurement $M_j$.

The two rotations, each through $2\pi$ have the combined effect of flipping the signs of the states $|1\rangle$ and $|2\rangle$ relative to state $|3\rangle$, specifically, we have:

$$|F\rangle = \hat{U}_{IF}|I\rangle \tag{15}$$

therefore by applying these two rotations, Alice can map $|F\rangle \rightarrow |I\rangle \rightarrow |3\rangle$, and measure $M_3$ as per the main text.

## PROBABILITY NOTATION FOR CLASSICAL MODELS OF THE THREE BOX PROBLEM

A basic classical models of the 'three-box' problem can be constructed[6] by assuming that the system of three boxes exists at all times in a definite state of having one box occupied and the other two empty. The classical state is conventionally labelled '$\lambda$'. The simplest classical model of three boxes sharing one ball assumes a one-to-one correspondence between the system states $\lambda_j$ and the available measurements $M_j$; so that if $\lambda$ is known, all measurement results can be inferred with certainty. The system with three states $\lambda_1$, $\lambda_2$, and $\lambda_3$, behaves so that being in state $\lambda_j$ corresponds to finding $M_j$-true and $M_{k\neq j}$-false. We can also assume many equivalent microstates $\{\lambda_1, \lambda_1', \lambda_1'', \cdots\}$ exist, that produce identical results when studied with the $M_j$ measurements. This situation is illustrated in figure 1

**Extensions of the classical model**

We can envisage extensions to the simple classical model presented above. Suppose that prior to measurement, the system is in a *definite* state $\lambda_i$ which however has the property of responding 'true' to more than one $M_j$ measurement on a statistical basis; for instance in the illustration of figure 2, the state $\lambda_i$ will answer 'true' with 1/3 probability to each of the $M_1$, $M_2$ and $M_3$ measurements. The state $\lambda_i$ is a definite state, distinct from a statistical mixture of $\lambda_1$, $\lambda_2$ and $\lambda_3$. In some sense $\lambda_i$ mimics the superposition state $|I\rangle = (|1\rangle + |2\rangle + |3\rangle)/\sqrt{3}$ prepared by Alice in the quantum version of the game.

We do not investigate whether an extended classical model can accurately describe the three-box problem in full detail, but to anticipate the possibility of such an extended classical model including states such as $\lambda_i$, we adopt a notation where the probability, given that we have performed measurement $M_j$, of obtaining the result 'true' is written $P_{M_j}(\text{true}) = \cdots$. This contrasts with simply writing $P(M_3) = \cdots$, which is adequate when all states $\lambda$ correspond to definite measurement outcomes, as assumed for the simplest classical model.

Specifically, we write the probability that Alice has seen her final $M_3$-result true, given that Bob had earlier performed $M_1$ and found his $M_1$-result true as the intersection of A-true and B-true given measurement context $M_1$:

$$P_{M_1}(A \cap B) = \cdots \tag{16}$$

Since Alice always performs $M_3$, we drop the suffix that would indicate the choice of her measurement, and only Bob's measurement is labelled. Likewise the probability that Alice has seen her final $M_3$-result true, given that Bob had earlier performed $M_2$ and found his $M_2$-result true is written:

$$P_{M_2}(A \cap B) = \cdots \tag{17}$$

The probability that Alice finds her $M_3$-result true, given that Bob had performed $M_1$ and found his $M_1$-result false is written:

$$P_{M_1}(A \cap \neg B) = \cdots \tag{18}$$

Alice and Bob can each either find their measurement results 'true' or 'false'. We must therefore have:

$$P_{M_j}(A \cap B) + P_{M_j}(A \cap \neg B) + P_{M_j}(\neg A \cap B) + P_{M_j}(\neg A \cap \neg B) = 1 \tag{19}$$

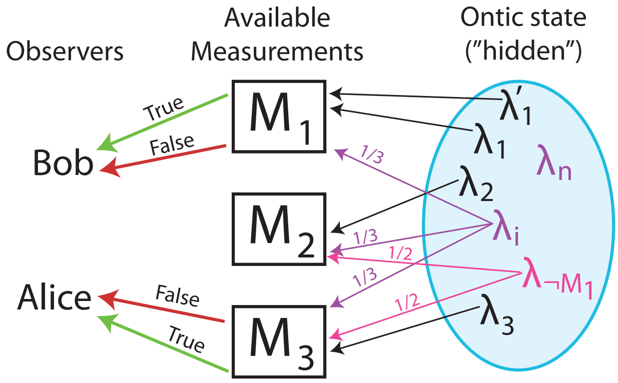


FIG. 2. **An extension of the classical model of the three-box problem.** We assume the existence of states $\lambda_i$ and $\lambda_{\neg M_1}$ that do not correspond to observable states such as the ball in a unique box, but that 'collapse' on measurement in a manner resembling quantum mechanics.

In the main text of the article, we show that $P_{M_j}(A \cap \neg B) = 0$ for both $j = 1$ and $j = 2$, under the quantum game.

## THE MACROREALIST ANALYSIS

In the macrorealist picture, finding the system in state $j$ corresponds to finding a macroscopic object, such as a hidden ball, in location such as box $j$. We write probabilities $P_{M_j}(B)$ to indicate the chance that when Bob performs measurement $M_j$ he sees a full box (finds state $j$) and $P_{M_j}(\neg B)$ as the probability that he finds box $j$ is empty (measures "not state $j$"). The probability of the combined event where both Bob and Alice see full boxes (both find state $j$) under measurement $M_j$ is $P_{M_j}(B \cap A) = P_{M_j}(B|A)P_{M_j}(A)$ while Alice's result when Bob makes no measurement is written $P_N(A)$.

The probabilities $P_{M_j}(\cdots)$ and $P_N(\cdots)$ are well-defined in both quantum and macrorealist theories, but our objective is to highlight the differences between these two theoretical descriptions. A macrorealist further believes that 'counterfactual' expressions take a definite value. He defines quantities such as $\tilde{P}_{\tilde{M}_j}(B)$ that give the probability for Bob to have found the object, had he performed $M_j$. This allows a macrorealist to insert a resolution of the identity into his expressions for probabilities as:

$$\tilde{P}_{\tilde{M}_1}(B) + \tilde{P}_{\tilde{M}_2}(B) + \tilde{P}_{\tilde{M}_3}(B) = 1 \tag{20}$$

wherever he chooses. (We track quantities that are undefined in quantum mechanics with tilde symbols)

**Deriving a Leggett-Garg Inequality specific to the 'Three Box' problem**

The Leggett-Garg (LG) function $K$ is a test for consistency with macrorealism[1]. It is characterised by three time-separated measurements $Q_1$, $Q_2$, $Q_3$ evaluated in pairs, so that:

$$\langle K\rangle = \langle Q_1 Q_2\rangle + \langle Q_2 Q_3\rangle + \langle Q_1 Q_3\rangle \tag{21}$$

Individually, each $Q_j$ measurement is a true ($Q_j = +1$) or false ($Q_j = -1$) statement about the system; the corresponding quantum mechanical operators $\hat{Q}_j$ take eigenvalues $\pm 1$.

In the framework of macrorealism, if only non-detectable (ND) measurements are performed, each $Q_j$ may take a value independent of the measurement sequence or Bob's choice of $j$, and the LG function then describes a sum of three parity checks from which at most two may be negative[2]. The LG function therefore falls in the range $-1 \leq \langle K\rangle \leq 3$ for an MR description of any system, but it may fall outside this range under quantum mechanics (or potentially other theories), indicating when experimental systems are incompatible with the MR picture.

We apply the LG analysis to our system as follows: Our experiment uses measurement based initialisation[3] to prepare the initial state, and we can take $Q_1 = +1$ in all cases. We assign $Q_2 = -1$ whenever Bob observes the object in box 1 or box 2 and $Q_2 = +1$ whenever he should infer the object is in box 3. We assign $Q_3 = +1$ whenever Alice's final $M_3$-result is true and assign $Q_3 = -1$ whenever the $M_3$-result is false.

If the macrorealist framework is applicable, one of six possible measurement histories $(a - f)$ must account for each particular run of the experiment (See table I). To assign the probabilities that a given history occured, the macrorealist must calculate the unobserved quantities $\tilde{P}_{\tilde{M}_3}(B \cap A)$ and $\tilde{P}_{\tilde{M}_3}(B \cap \neg A)$. If the measurements are operationally non-disturbing (a property that we check experimentally), it is possible to substitute $\tilde{P}_{\tilde{M}_1}(B|A) \Rightarrow P_{M_1}(B|A)$ and $\tilde{P}_{\tilde{M}_2}(B|A) \Rightarrow P_{M_2}(B|A)$ (*etc.*) for the measurements that are made, so that:

$$\tilde{P}_{\tilde{M}_3}(B) = 1 - P_{M_1}(B) - P_{M_2}(B) \tag{22}$$

$$\tilde{P}_{\tilde{M}_3}(B \cap A) = P_N(A) - P_{M_1}(B \cap A) - P_{M_2}(B \cap A) \tag{23}$$

$$\tilde{P}_{\tilde{M}_3}(B \cap \neg A) = P_N(\neg A) - P_{M_1}(B \cap \neg A) - P_{M_2}(B \cap \neg A) \tag{24}$$

| Case | $Q_1$ | Bob measures: | $Q_2$ | Alice measures: | $Q_3$ | $K$ | Probability |
|---|---|---|---|---|---|---|---|
| a | $+1$ | $M_1$ | $-1$ | $M_3$ | $+1$ | $-1$ | $P_{M_1}(B \cap A)$ |
| b | $+1$ | $M_2$ | $-1$ | $M_3$ | $+1$ | $-1$ | $P_{M_2}(B \cap A)$ |
| c | $+1$ | infers $M_3$ | $+1$ | $M_3$ | $+1$ | $+3$ | $\tilde{P}_{\tilde{M}_3}(B \cap A)$ |
| d | $+1$ | $M_1$ | $-1$ | $\neg M_3$ | $-1$ | $-1$ | $P_{M_1}(B \cap \neg A)$ |
| e | $+1$ | $M_2$ | $-1$ | $\neg M_3$ | $-1$ | $-1$ | $P_{M_2}(B \cap \neg A)$ |
| f | $+1$ | infers $M_3$ | $+1$ | $\neg M_3$ | $-1$ | $-1$ | $\tilde{P}_{\tilde{M}_3}(B \cap \neg A)$ |

TABLE I. The assignment $Q_j$ values for each run of the experiment. According to the MR picture, one of the six cases above must account for each run of the experiment. The measured probabilities $P_{M_1}$ and $P_{M_2}$ and inferred (counterfactual) probabilities $\tilde{P}_{\tilde{M}_3}$ that weight the value of $K$ corresponding to each history are listed in the table above.

Using these definitions, the macrorealist framework deduces the expression for $\langle K \rangle$ (see table I) as:

$$\begin{aligned} \langle K \rangle = &- P_{M_1}(B \cap A) - P_{M_2}(B \cap A) + 3\tilde{P}_{\tilde{M}_3}(B \cap A) \\ &- P_{M_1}(B \cap \neg A) - P_{M_2}(B \cap \neg A) - \tilde{P}_{\tilde{M}_3}(B \cap \neg A) \end{aligned} \tag{25}$$

which in terms of observable quantities is:

$$\begin{aligned} \langle K \rangle = &- P_{M_1}(B \cap A) - P_{M_1}(B \cap \neg A) \\ &- P_{M_2}(B \cap A) - P_{M_2}(B \cap \neg A) \\ &+ 3P_N(A) - 3P_{M_1}(B \cap A) - 3P_{M_2}(B \cap A) \\ &- P_N(\neg A) + P_{M_1}(B \cap \neg A) + P_{M_2}(B \cap \neg A) \end{aligned} \tag{26}$$

This expression simplifies to:

$$\langle K \rangle = 4P_N(A) - 4P_{M_1}(B \cap A) - 4P_{M_2}(B \cap A) - 1 \tag{27}$$

We know that the quantum expressions for these occurrences are:

$$P_N(A) = |\langle F|I\rangle|^2 = 1/9 \tag{28}$$

$$P_{M_1}(B \cap A) = |\langle F|\hat{P}_1|I\rangle|^2 = 1/9 \tag{29}$$

$$P_{M_2}(B \cap A) = |\langle F|\hat{P}_2|I\rangle|^2 = 1/9 \tag{30}$$

We observe two points here; given the probabilities above **a)** Alice is unable to determine whether Bob has chosen to perform measurement $M_1$, measurement $M_2$ or neither measurement ($N$) and that Alice's result is independent of measurement context. We have:

$$P_{M_1}(A) = P_{M_2}(A) = P_N(A) \tag{31}$$

Further, **b)** we have that:

$$P_{M_1}(\neg B \cap A) = P_{M_2}(\neg B \cap A) = 0 \tag{32}$$

Alice will never find her $M_3$-result true, when Bob has found his $M_j$-result false, the key feature that enables Alice to win the three-box game. This implies:

$$P_{M_1}(B \cap A) = P_{M_1}(A) \tag{33}$$

$$P_{M_2}(B \cap A) = P_{M_2}(A) \tag{34}$$

We can extract the probability of Alice's measurement from each term via Bayes theorem

$$P(B \cap A) = P(B|A)P(A) \tag{35}$$

yielding:

$$\begin{aligned} \langle K \rangle &= 4P(A)(1 - P_{M_1}(B|A) - P_{M_2}(B|A)) - 1 \\ &= \frac{4}{9}(1 - P_{M_1}(B|A) - P_{M_2}(B|A)) - 1 \end{aligned} \tag{36}$$

Given the macrorealist's hypothesis, the events under $M_1$ and $M_2$ should be mutually exclusive, and sums of events under these cases will obey an inequality:

$$P_{M_1}(\cdots) + P_{M_2}(\cdots) \leq 1 \tag{37}$$

The equality holds when the Leggett-Garg function in eqation 36 takes it's limiting value $\langle K \rangle = -1$. In the quantum case meanwhile, $P_{M_1}(\cdots)$ and $P_{M_2}(\cdots)$ are independent, and we have:

$$P_{M_1}(\cdots) + P_{M_2}(\cdots) \leq 2 \tag{38}$$

allowing the Leggett-Garg function to reach a value of:

$$\langle K \rangle = -\frac{13}{9} = -1.4\dot{4} \tag{39}$$

This is outside the range $-1 \leq \langle K \rangle \leq 3$ providing an opportunity to detect an inconsistency with macrorealism.

## EXPERIMENTAL IMPLEMENTATION OF NUCLEAR SPIN READOUT

### Sample

We use a naturally occurring nitrogen-vacancy (NV) centre in high purity (spin-bearing impurities controlled below 1 part per billion) type IIa diamond grown by chemical vapour deposition, with a $\langle 111 \rangle$ crystal orientation obtained by cleaving a $\langle 100 \rangle$ substrate. We optimise the photon collection efficiency through use of a solid immersion lens deterministically fabricated by focussed ion beam milling[4] to focus light onto the selected NV centre. Microwave and radio frequency pulses for the spin manipulation are applied through a lithographically defined stripline adjacent to the solid immersion lens[4].

### Measurement Setup

We use a home-built low-temperature confocal microscope that has been described in detail in Robledo[3] *et al.* All experiments are performed at a sample temperature of T=8.7 K. A small magnetic field (B $\approx$ 5 G, oriented along the NV symmetry axis) is applied by means of four permanent magnets arranged around the cryostat.

### General

In the course of this experiment, we use different variations of single-shot nuclear spin readout, adapted to our specific purpose. In general, nuclear spin readout is implemented according to the following protocol[3]:

1. Optional: Electron spin initialization by optical pumping into $m_S = 0$ (excitation of $A_1$ transition) or $m_S = \pm 1$ (excitation of $E_x$ transition)

2. Map nuclear spin onto electron spin: Selective MW excitation of the hyperfine transition representing the state to be probed (in general, effecting a $\pi$ rotation)

3. Readout of the electron spin: Resonant optical excitation on $E_x$ transition (for maximum contrast, $t_{ro} \approx 15 - 25\,\mu$s).

4. Optional: Restore the electron spin state by optical pumping (for deterministic preparation of $m_S = +1$ or $m_S = -1$: optical pumping into $m_S = 0$, followed by a MW $\pi$-pulse)

If readout of the electron spin yields a result different than its initial state, we conclude that the nuclear spin occupies the probed state. The readout can be repeated using different MW frequencies, allowing us to perform population tomography on the full electron-nuclear spin state. We now outline the readout variations used.

**Nuclear spin initialization**

Initialization of the $^{14}$N nuclear spin into $m_I = 0$ represents the first measurement of the Leggett-Garg test $Q_1$. This first measurement is probabilistic - we choose parameters that maximise the preparation fidelity with respect to the post-measurement state, accepting a reduced preparation success probability.

- The electron spin is initialised in the $m_S = \pm 1$ manifold by optical pumping, implemented by a pulse of $200\,\mu s$ duration, resonant with the $E_x$ transition (fidelity $F = 99.4\%$). The initialization fidelity is further increased to $F > 99.9\%$ by postselecting only experimental runs where no photon is detected during the last $50\,\mu$s of the optical pumping pulse (avoiding accidental re-population of $m_S = 0$).

- We then apply a MW $\pi$-pulse resonant with the transition $|m_S = -1, m_I = 0\rangle \rightarrow |m_S = 0, m_I = 0\rangle$ with a state selectivity of $\approx 98\%$, limited by proximity of other hyperfine transitions.

- We probe successful initialization into $m_I = 0$ by requiring $> 0$ detected photons during $E_x$ excitation. To maximise fidelity, we keep the readout duration short (200 ns).

- During the electron spin readout there is a finite chance of optically induced electron spin flips. To ensure the electron to occupy the $m_S = -1$ state, we first optically pump it into $m_S = 0$, and then apply a selective MW $\pi$-pulse resonant with $|m_S = 0, m_I = 0\rangle \rightarrow |m_S = -1, m_I = 0\rangle$.

- after succesful initialization we estimate an overlap with $|m_S = -1, m_I = 0\rangle$ of $> 95\%$.

All runs of the three-box experiment use this initialization step.

### Three Box Game: Bob's readout

The second readout (Bob's readout) consists of a selective MW $\pi$-pulse, resonant with:

$$|m_S = -1, m_I = -1\rangle \rightarrow |m_S = 0, m_I = -1\rangle \qquad (M_1) \tag{40}$$

$$|m_S = -1, m_I = +1\rangle \rightarrow |m_S = 0, m_I = +1\rangle \qquad (M_2) \tag{41}$$

$$|m_S = -1, m_I = 0\rangle \rightarrow |m_S = 0, m_I = 0\rangle \qquad (M_3) \tag{42}$$

depending on Bob's choice of measurement. Subsequently, the electron spin state is probed by a $t_{ro} = 20\,\mu$s pulse resonant with $E_x$. This readout gives a large contrast (fidelity 96%), but if $m_S = 0$ is detected, many excitation cycles may have occurred, and due to optically induced spin flips the electron spin may be left in an undefined state. As a remedy, conditional on obtaining an $m_S = 0$ readout result, we restore the spin into $m_S = -1$ by optical pumping into $m_S = 0$, followed by a selective MW $\pi$-pulse, $|m_S = 0, m_I = +1(-1)\rangle \rightarrow |m_S = -1, m_I = +1(-1)\rangle$ $(M_{1(2)})$. This procedure ensures to find the electron deterministically in $m_S = -1$ after the readout, leaving nuclear spin coherence unaffected.

### Three Box Game: Alice's readout

While for the last readout (Alice's readout) we could in principle apply the same protocol as in Bob's readout, we decided to read out all three nuclear spin states (box states) for each measurement – allowing us to also identify the few cases where we don't find the ball in any of the boxes (e.g. to determine the finite detection efficiency of the nuclear spin readout).

For each probed nuclear spin state, we repeat two readout iterations consisting of a selective MW $\pi$-pulse and a $20\,\mu$s $E_x$ readout pulse. This is repeated for the three hyperfine lines corresponding to the $m_S = -1$ manifold (implementing $M_1$, $M_2$ and $M_3$). The first probed state found to emit a photon is identified as the readout result; if no photon is detected, we consequently assign no result. To avoid a readout bias due to order of the probed states, we permute the order between measurements.

### Probing the initial state $|I\rangle$

To test successful generation of state $|I\rangle = \frac{1}{\sqrt{3}}(|1\rangle + |2\rangle + |3\rangle)$ (data in Fig. 3 a,i), we show data from Bob's readout of the 3-box-game, with 1200 repetitions of measuring each

$M_1$, $M_2$ and $M_3$.

### Probing repeatability

Data shown in Fig. 3 a, ii-iii and Fig. 3 b,c is obtained by correlating two successive readouts, implemented as Bob's and Alice's readout in the '3-box-game'. However, here we omit the NMR manipulation between Bob's and Alice's readout, so both readout instances probe in the same basis. For each choice of Bob's measurement ($M_1$, $M_2$ or $M_3$), in the following readout we probe all nuclear spin states within the $m_S = -1$ manifold in the same measurement run.

## ERROR ANALYSIS

We find small deviations from the values expected from an ideal implementation. In the following, we give a brief description of the origin of these discrepancies and discuss their consequences on the macrorealist's possible conclusions.

1. We find $\sum_j P_{M_j}(B) < 1$, i.e. there is not always a ball found in all of the boxes. This is a consequence of a smaller than unity probability of correctly identifying the electronic $m_S = 0$ state, resulting in an effective detection efficiency of $P_{det} \approx 90\%$. While the macrorealist might conclude that there is not always an object hidden in the boxes, he still finds an unbiased initial state (within statistical uncertainty). Therefore he cannot expect Alice to take advantage of this discrepancy – based on his secret choice of $M_1$ or $M_2$ and the reduced probability to find an object, he expects a maximum probability of $\frac{P_{det}}{2} \leq \frac{1}{2}$ of Alice predicting his positive measurement outcome correctly, so the macrorealist finds an even stronger violation of his expectations.

2. For sequential measurements $i$, $i{+}1$, we find both $P(M_{j,i+1}|M_{j,i})$ and $P(\neg M_{j,i+1}|\neg M_{j,i})$ $< 100\%$ (Fig. 3b), i.e. after measuring its position, with a small probability the object is moved to a different box. This finding could indeed explain correlations between Bob's and Alice's measurements: As a worst-case scenario, Bob could assume a hidden mechanism in the game whereby Bob's successful measurement 'moves' the object, deterministically storing it in the box Alice is probing and maximizing her conditional

probability $P_{M_j}(B|A)$. He would deduce an upper limit for her success probability of $P_{M_j}(B|A) \leq \frac{1}{3} + P(\text{object moves})$. Taking into account all "Changed" and "Undetermined" events (Fig. 3b), he finds $P(\text{object moves}) \leq 28\%$, and $P_{M_j}(B|A) \leq 61\%$, clearly violated by the experimental findings.

3. We find $P(A) \approx 14\% > 1/9$ (Fig. 4a). However from the QM description we expect:

$$P_N(A) = |\langle F|I\rangle|^2 = 1/9 \tag{43}$$

$$P_{M_1}(B \cap A) = |\langle F|\hat{P}_1|I\rangle|^2 = 1/9 \tag{44}$$

$$P_{M_2}(B \cap A) = |\langle F|\hat{P}_2|I\rangle|^2 = 1/9 \tag{45}$$

In our implementation, between measurement $A$ and $B$ we apply the transformation $|F\rangle \rightarrow |I\rangle \rightarrow |3\rangle$, consisting of NMR pulses of a total duration of $\approx 750\,\mu$s. RF-induced heating of the sample and nuclear spin dephasing limits the fidelity of this operation, leading to an increased probability $P(A)$. In the QM picture, Alice detects more positive results than she should (unconditional on measurement $B$), thus her conditional probability $P_{M_j}(B|A)$ to correctly predict Bob's measurement outcome must drop below the theoretical maximum of 100% (Fig. 4b).

## STATISTICAL ERROR ANALYSIS

For each particular run of our experiment, we can either count one or more photons ($n \geq 1$) or no photons ($n = 0$), inferring that the electron is in the $m_S = 0$ or $m_S = \pm 1$ state. A detailed analysis of the inferences between photon number and spin state were presented by Robledo *et al.*[3] as a combination geometric distribution (accounting for the spin flip rate), binomial distribution (accounting for photon detector efficiency) and the poissonian background rate. For the purposes of our analysis, we define a variable $p = |m_S|$ which is the value of Bob or Alice's $M_j$-result on any particular round of the experiment. We assign $p = 0$ when we count $n = 0$ photons, and assign $p = 1$ when we count $n \geq 1$ photons. We then define the probability $p$ to find $m_S = 0$ during a particular shot of the experiment as

$f$, so that during $N$ trials of the experiment we expect to observe statistics:

$$\text{Mean}\,[p] = Nf \tag{46}$$

$$\text{Var}\,[p] = \sigma^2(p) = Nf(1-f) \tag{47}$$

$$\text{Std.Dev.}\,[p] = \sigma(p) = \sqrt{Nf(1-f)} \tag{48}$$

We use this to calculate the statistical significance of our results (e.g. the chance that the Leggett-Garg function we measured is compatible with macrorealism, and that counting statistics have produced a violation by chance).

## FAIR SAMPLING VS. ADVERSARIAL MACROREALIST POSITIONS

In our experiment, we have the option to measure either the population in electron spin sublevel $m_S = -1$ or the electron spin sublevels $m_S = -1$ and $m_S = +1$ when performing Bob and Alice's measurements $M_j$. Measuring the $m_S = -1$ populations only, we have a the possibility to obtain 'undetermined' outcomes in which the population branches from $m_S = -1$ to the uninspected $m_S = +1$ levels during measurement, whilst by measuring the $m_S = -1$ and $m_S = +1$ levels, we minimise these undetermined events, whilst increasing the number of $\Delta m_I$ nuclear spin flips which correspond to Bob measuring that the state has definitely changed between subsequent measurements.

There are two approaches that we could use to interpret the 'undetermined' outcomes. The default assumption is that the unmeasured values are distributed fairly, and will follow the same distribution as the measured values, whereas the most extreme assumption is that each unmeasured value somehow represents Alice 'cheating' by hiding values that favour the macrorealist hypothesis. If we take this extreme position, it is interesting to know whether a result compatible with macrorealism could be recovered, by allowing Bob to assign a value to each "undetermined" result as he pleases[5]. We then define quantities such as:

$$P(A \cap B)^{\text{min}}_{M1} = \frac{N_{M1}(B \cap A)}{N_{M1}(B \cap A) + N_{M1}(\neg B \cap A) + N_{M_1}(U)} \tag{49}$$

$$P(A \cap B)^{\text{fair}}_{M1} = \frac{N_{M1}(B \cap A)}{N_{M1}(B \cap A) + N_{M1}(\neg B \cap A)} \tag{50}$$

$$P(A \cap B)^{\text{max}}_{M1} = \frac{N_{M1}(B \cap A) + N_{M_1}(U)}{N_{M1}(B \cap A) + N_{M1}(\neg B \cap A) + N_{M_1}(U)} \tag{51}$$

Where $N_{M_1}(U)$ is the number of undetermined measurement readings, given that Bob has performed $M_1$. This bounds the possibilities for Bob to reassign undetermined readings. In

fact, both in the case where we assume fair sampling, and without, we find that $\langle K \rangle \leq -1$, and that our results are therefore incompatible with macrorealism. We calculate each case and include errors as per our statistical analysis above. In the case that we include only $m_S = -1$ read-out, we find:

$$K^{\text{min}}_{|m_S=-1} = -1.2026 \qquad \sigma^{\text{min}}_{|m_S=-1} = 0.0259 \qquad (7.81\,\sigma \text{ violation}) \tag{52}$$
$$K^{\text{fair}}_{|m_S=-1} = -1.2647 \qquad \sigma^{\text{fair}}_{|m_S=-1} = 0.0234 \qquad (11.29\,\sigma \text{ violation}) \tag{53}$$
$$K^{\text{max}}_{|m_S=-1} = -1.3494 \qquad \sigma^{\text{max}}_{|m_S=-1} = 0.0173 \qquad (20.19\,\sigma \text{ violation}) \tag{54}$$

Whilst using the complete register read-out on $m_S = -1$ and $m_S = +1$ we have:

$$K^{\text{min}}_{|m_S=\pm1} = -1.1373 \qquad \sigma^{\text{min}}_{|m_S=\pm1} = 0.0252 \qquad (5.46\,\sigma \text{ violation}) \tag{55}$$
$$K^{\text{fair}}_{|m_S=\pm1} = -1.1833 \qquad \sigma^{\text{fair}}_{|m_S=\pm1} = 0.0241 \qquad (7.60\,\sigma \text{ violation}) \tag{56}$$
$$K^{\text{max}}_{|m_S=\pm1} = -1.2531 \qquad \sigma^{\text{max}}_{|m_S=\pm1} = 0.0210 \qquad (12.07\,\sigma \text{ violation}) \tag{57}$$

In the event, we found that the undetermined measurement outcomes do not give Bob sufficient leeway to explain the discrepancy of our result from the range predicted by macro-realism, even when taking the most adversarial position permissible with respect to our data.

---

* richard.george@materials.ox.ac.uk

† l.m.robledoesparza@tudelft.nl

[1] Leggett, A. & Garg, A. Quantum-Mechanics Versus Macroscopic Realism - Is the Flux There When Nobody Looks? *Phys. Rev. Lett.* **54**, 857–860 (1985).

[2] Vaidman, L. An Impossible Necklace. In Bertlmann, R. & Zeilinger, A. (eds.) *Quantum [Un]speakables: From Bell's Theorem to Quantum Information*, 221–223 (Springer, 2002).

[3] Robledo, L. *et al.* High-fidelity projective read-out of a solid-state spin quantum register. *Nature* **477**, 574–578 (2011).

[4] Bernien, H. *et al.* Two-Photon Quantum Interference from Separate Nitrogen Vacancy Centers in Diamond. *Phys. Rev. Lett.* **108**, 043604 (2012).

[5] Knee, G., Simmons, S., Gauger, E. & Morton, J. Violation of a Leggett-Garg inequality with ideal non-invasive measurements. *Nature Communications* (2012).

[6] N.B. such models cannot describe Alice's ability to win the game on $\geq 50\%$ of rounds.
